# Supplementary material for: Structured Mappings and Conferencing Common Information for Multiple-access Channels
Source: arXiv:1905.04760 source file (2019-05-12)
Supplement: Supplementary file 1 [file MAC_Corr_Scr_Appendices.tex]

\section{Proof of Theorem \ref{them: achievable-rate-for -proposed scheme}}\label{sec: proof of them lin_ces}
\begin{proof}
There are two error events, $E_0$ and $E_1$. $E_0$ occurs if no $\underline{\mathbf{\tilde{s}}}$ was found. $E_1$ is declared if  $\underline{\mathbf{\tilde{s}}} \neq \underline{\mathbf{s}}$. To show that $E_0$ is small, we need the next lemma. Suppose $v_i()$ and $v_i()$ are a realization of random functions generated as in the outline of the proof of Theorem \ref{them: achievable-rate-for -proposed scheme}.

\begin{lem}\label{len: prob jth comp}
Suppose $\mathbf{s}_i, i=1,2,3$ are jointly typical with respect to $P_{\underline{\mathbf{S}}}$. Then 
\begin{align*}
\big(&v_1(\mathbf{s}_1),v_2(\mathbf{s}_2), v_3(\mathbf{s}_3),x_1(\mathbf{s}_1,v_1(\mathbf{s}_1)), \\& x_2(\mathbf{s}_2,v_2(\mathbf{s}_2)),x_3(\mathbf{s}_3,v_3(\mathbf{s}_3))\big)\in A_{\epsilon}^{(n)}(V_1V_2V_3X_1X_2X_3|\mathbf{s}_1\mathbf{s}_2 \mathbf{s}_3).
\end{align*}

%
%\begin{align*}
%P\{\mathbf{v}_i=\Phi_i(\mathbf{s}_i), \mathbf{x}_i=\mathbf{X}_i(\mathbf{s}_i, \mathbf{v}_i)  \mbox{for } l=1,2,3\}=\frac{1}{2^{2n}}\prod_{j=1}^n p(v_{3j}|v_{1j}, v_{2j},s_{1j}, s_{2j},s_{3j}) p(x_{1j}|s_{1,j}v_{1j})p(x_{1j}|s_{1,j}v_{1j})
%\end{align*}
\end{lem}
\begin{proof}
The proof is straightforward. 
\end{proof}
As a result, the sequences $\mathbf{s}_i, \mathbf{v}_i, \mathbf{x}_i, i=1,2,3$ are jointly typical with $\mathbf{y}$ with respect to $P_{\underline{\mathbf{S}}, \underline{\mathbf{V}}, \underline{\mathbf{X}},Y}$. This implies that  $P(E_0)$ approaches $0$ as $n \rightarrow \infty$. Next, we calculate $P(E_1 \cap E_0^c)$. For a given $\underline{\mathbf{s}}\in A_{\epsilon}(\underline{S})$, using the definition of $E_1$ and the union bound we obtain,
\begin{align*}
P(E_1 \cap E_0^c|\underline{\mathbf{s}}) \leq &  \sum_{ (\underline{\mathbf{v}},\underline{\mathbf{x}})\in  A_{\epsilon}(\underline{\mathbf{V}},\underline{\mathbf{X}}|\underline{\mathbf{s}})} \mathbbm{1}\{\mathbf{v}_i=v_i(\mathbf{s}_i), \mathbf{x}_i=x_i(\mathbf{s}_i, \mathbf{v}_i), ~ i=1,2,3\} \sum_{\mathbf{y}\in A_{\epsilon}(Y|\underline{\mathbf{x}})}p(\mathbf{y}|\underline{\mathbf{x}})\\
 &\sum_{\substack{(\underline{\mathbf{\tilde{s}}},\underline{\tilde{\mathbf{v}}},\underline{\tilde{\mathbf{x}}})\in A_{\epsilon}(\underline{S},\underline{V},\underline{X}|\mathbf{y})\\ \underline{\tilde{\mathbf{s}}} \neq \underline{\mathbf{s}}}} \mathbbm{1}\{\tilde{\mathbf{v}}_j=v_j(\tilde{\mathbf{s}}_j), \tilde{\mathbf{x}}_j=x_j(\tilde{\mathbf{s}}_j, \tilde{\mathbf{v}}_j), j=1,2,3\}
\end{align*}

Taking expectation over random functions  $X_i(,)$ and $V_i()$ gives,
\begin{align}\label{eq: Pe}
p_e(\underline{\mathbf{s}})&=\EE\{P(E_{1}|\underline{\mathbf{s}})\} \leq   \sum_{(\underline{\mathbf{v}}, \underline{\mathbf{x}},\mathbf{y})\in A_{\epsilon}(\underline{V}, \underline{X},Y|\underline{\mathbf{s}})} p(\mathbf{y}|\underline{\mathbf{x}})
 \sum_{\substack{(\underline{\mathbf{\tilde{s}}},\underline{\tilde{\mathbf{v}}},\underline{\tilde{\mathbf{x}}})\in A_{\epsilon}(\underline{S},\underline{V},\underline{X}|\mathbf{y})\\ \underline{\tilde{\mathbf{s}}} \neq \underline{\mathbf{s}}}} \\ \nonumber
& P\{\mathbf{v}_l=V_l(\mathbf{s}_l), \mathbf{x}_l=X_l(\mathbf{s}_l, \mathbf{v}_l), \tilde{\mathbf{v}}_l=V_l(\tilde{\mathbf{s}}_l), \tilde{\mathbf{x}}_l=X_l(\tilde{\mathbf{s}}_l, \tilde{\mathbf{v}}_l) ~ \mbox{for } l=1,2,3\}
\end{align}
%We need the following Lemma to proceed.

Note that $V_i()$ and $\mathbf{X}_i(~,~)$ are generated independently. So the most inner term in (\ref{eq: Pe}) is simplified to 
\begin{align}\label{eq: pp 1}
P\{\mathbf{v}_j=V_j(\mathbf{s}_j), \tilde{\mathbf{v}}_j=V_j(\tilde{\mathbf{s}}_j)~ j=1,2\} P\{\mathbf{x}_l=X_l(\mathbf{s}_l, \mathbf{v}_l), \tilde{\mathbf{x}}_l=X_l(\tilde{\mathbf{s}}_l, \tilde{\mathbf{v}}_l) ~  l=1,2,3\}.
\end{align}
Note $j=3$ is redundant because, $\mathbf{v}_3 = \mathbf{v}_1\oplus_q \mathbf{v}_2$ and $\mathbf{\tilde{v}}_3 = \mathbf{\tilde{v}}_1\oplus_q \mathbf{\tilde{v}}_2$. By definition, $V_j(\mathbf{s}_j)=\mathbf{s}_j\mathbf{G}+\mathbf{B}_j, j=1,2$, where $B_1,B_2$ are uniform and  independent of $\mathbf{G}$. Then 
\begin{align}\label{eq: PP 2}
P\{\mathbf{v}_j=\Phi_j(\mathbf{s}_j), \tilde{\mathbf{v}}_j=\Phi_j(\tilde{\mathbf{s}}_j)~ j=1,2\} = \frac{1}{q^{2n}} P\{(\tilde{\mathbf{s}}_j-\mathbf{s}_j)\mathbf{G}=\tilde{\mathbf{v}}_j-\mathbf{v}_j, ~j=1,2\}
\end{align}
The following lemma determines the above term.
\begin{lem}\label{lem: prob of sG}
Suppose elements of $\mathbf{G}$ are generated randomly and uniformly from $\FF_q$. If $\mathbf{s}_1$ or $\mathbf{s}_2$ is nonzero, the following holds: 
\begin{align*}
P\{\mathbf{s}_j\mathbf{G}=\mathbf{v}_j, ~j=1,2\}= \left\{ \begin{array}{ll}
%\mathbbm{1}\{\mathbf{v}_j=\mathbf{0}, ~ l=1,2\}, & \mbox{if}~ \mathbf{s}_1 = \mathbf{0},  \mathbf{s}_2=\mathbf{0}.\\
q^{-n}\mathbbm{1}\{\mathbf{v}_j=\mathbf{0}\} , & \mbox{if}~ \mathbf{s}_j=\mathbf{0}\\
%q^{-n}\mathbbm{1}\{\mathbf{\tilde{v}}_1=\mathbf{v}_1\} , & \mbox{if}~ \mathbf{\tilde{s}}_1 = \mathbf{s}_1,  \mathbf{\tilde{s}}_2\neq  \mathbf{s}_2.\\
q^{-n}\mathbbm{1}\{\mathbf{v}_1 = \mathbf{v}_2\}, & \mbox{if}~ \mathbf{s}_1 \neq \mathbf{0},  \mathbf{s}_2 \neq \mathbf{0}, \mathbf{s}_1= \mathbf{s}_2.\\
q^{-2n}, & \mbox{if}~ otherwise.\\
\end{array} \right.
\end{align*}
\end{lem}
\begin{proof}[Outline of the proof]
We can write $\mathbf{s}_j\mathbf{G}=\sum_{i=1}^n \mathbf{s}_{ji}\mathbf{G}_i$, where $\mathbf{s}_{ji}$ is the $i$th component of $\mathbf{s}_j$ and $\mathbf{G}_i$ is the $i$th row of $\mathbf{G}$. Not that $\mathbf{G}_i$ are independent random variables with uniform distribution over $\FF_q^n$. Hence, if $\mathbf{s}_j\neq \mathbf{0}$, then $\mathbf{s}_j\mathbf{G}$ is uniform over $\FF_q^n$. If $\mathbf{s}_1\neq \mathbf{s}_2$, one can show that $\mathbf{s}_1\mathbf{G}$ is independent of $\mathbf{s}_2\mathbf{G}$. The proof follows by arguing that if a random variables $X$ is independent of $Y$ and is uniform over $\FF_q$, then $X\oplus_q Y$ is also uniform over $\FF_q$ and is independent of $Y$. 
\end{proof}
Finally, we are ready to characterize the conditions in which $p_e\rightarrow 0$. We divide the last summation in (\ref{eq: Pe}) into the following cases:

\paragraph*{\bf Case 1, $\mathbf{\tilde{s}}_1 \neq \mathbf{s}_1,  \mathbf{\tilde{s}}_2= \mathbf{s}_2$}
In this case, using Lemma \ref{lem: prob of sG}, (\ref{eq: PP 2}) equals to $q^{-3n}\mathbbm{1}\{\mathbf{\tilde{v}}_2=\mathbf{v}_2\}$. Therefore, (\ref{eq: Pe}) is simplified to 
\begin{align*}
p_{e_1} (\underline{\mathbf{s}}) :=   \sum_{(\underline{\mathbf{v}}, \underline{\mathbf{x}},\mathbf{y})\in A_{\epsilon}(\underline{V}, \underline{X},Y|\underline{\mathbf{s}})} p(\mathbf{y}|\underline{\mathbf{x}})
 &\sum_{\substack{(\underline{\mathbf{\tilde{s}}},\underline{\tilde{\mathbf{v}}},\underline{\tilde{\mathbf{x}}})\in A_{\epsilon}(\underline{S},\underline{V},\underline{X}|\mathbf{y})\\ \underline{\tilde{\mathbf{s}}} \neq \underline{\mathbf{s}},  \mathbf{\tilde{s}}_2= \mathbf{s}_2,  \mathbf{\tilde{v}}_2= \mathbf{v}_2 }} 
q^{-3n}\\& P\{\mathbf{x}_l=\mathbf{X}_l(\mathbf{s}_l, \mathbf{v}_l), \tilde{\mathbf{x}}_l=\mathbf{X}_l(\tilde{\mathbf{s}}_l, \tilde{\mathbf{v}}_l) ~  l=1,2,3\}.
\end{align*} 

Note that $\mathbf{X}_l({\mathbf{s}}_l, \mathbf{{v}}_l)$ is independent of $\mathbf{X}_k(\tilde{\mathbf{s}}_k, \mathbf{\tilde{v}}_k)$, if $l \neq k$ or $\mathbf{s}_l \neq \mathbf{\tilde{s}}_l$ or $\mathbf{v}_l \neq \mathbf{\tilde{v}}_l$. Moreover, $P\{\mathbf{x}_l=\mathbf{X}_l(\mathbf{s}_l, \mathbf{v}_l)\}\approx 2^{nH(X_l|S_lV_l))}$.
As $\mathbf{s}_2=\mathbf{\tilde{s}}_2$ and $\mathbf{v}_2=\mathbf{\tilde{v}}_2$, then $X_2(\tilde{\mathbf{s}}_2, \tilde{\mathbf{v}}_2)=X_2(\mathbf{s}_2, \mathbf{v}_2)$. Therefore, 
\begin{align*}
P\{\mathbf{x}_l=X_l(\mathbf{s}_l, & \mathbf{v}_l), \tilde{\mathbf{x}}_l=X_l(\tilde{\mathbf{s}}_l, \tilde{\mathbf{v}}_l) ~  l=1,2,3\}\\&=2^{-n[2H(X_1|S_1V_1)+H(X_2|S_2V_2)+ 2H(X_3|S_3V_3)]} \mathbbm{1}\{\mathbf{\tilde{x}}_2=\mathbf{x}_2\}.
\end{align*}

Hence, we have:
\begin{align*}
p_{e_1}(\underline{\mathbf{s}})&\approx 2^{nH(\underline{V}, \underline{X}|\underline{S})} 2^{nH(S_1,V_1,X_1, S_3, V_3, X_3| Y S_2 V_2 X_2)} \frac{1}{q^{3n}}2^{-n[2H(X_1|S_1V_1)+H(X_2|S_2V_2)+2 H(X_3|S_3V_3)]}. 
\end{align*}
Note that $H(\underline{V},\underline{X}| \underline{S})=2\log_2q+\sum_{i=1}^3H(X_i|S_i,V_i)$. Therefore, $p_{e_1}\rightarrow 0$, if 
\begin{align}\label{eq: initial_inequality_case 1}
H(S_1,V_1,X_1, S_3, V_3, X_3| Y S_2 V_2 X_2)\leq \log_2q+ H(X_1|S_1V_1)+H(X_3|S_3V_3)
\end{align}
The right-hand side in the above inequality equals to $H(X_1X_3V_1V_3|S_1S_2S_3 X_2V_2)$. We simplify the left-hand side. Observe that $$H(S_1,V_1,X_1, S_3, V_3, X_3| Y S_2 V_2 X_2)=H(V_1,X_1, V_3, X_3| Y S_2 V_2 X_2)+H(S_1|S_2 \underline{V}~\underline{X}),$$
where $Y$ is removed from the second term, because conditioned on $\underline{X}$, $Y$ is independent of $S_1$. Note that
\begin{align*}
H(S_1|S_2 \underline{V}~\underline{X})&=H(S_1|S_2X_2V_2)-I(S_1;X_1V_1X_3V_3|S_2V_2X_2)\\&=H(S_1|S_2)-I(S_1;X_1V_1X_3V_3|S_2V_2X_2).
\end{align*}
Therefore, using the above argument the inequality in (\ref{eq: initial_inequality_case 1}) is simplified to
\begin{align*}
H(S_1|S_2)&\leq I(S_1;X_1V_1X_3V_3|S_2V_2X_2)-H(V_1,X_1, V_3, X_3| Y S_2 V_2 X_2)\\&+H(X_1X_3V_1V_3|S_1S_2S_3 X_2V_2)\\
%&=I(S_1;X_1V_1X_3V_3|S_2V_2X_2)-H(V_1,X_1, V_3, X_3| Y S_2 V_2 X_2)+H(X_1V_1X_3V_3|S_1S_2X_2V_2)\\
&=I(X_1V_1X_3V_3;Y|S_2V_2X_2)\\&=I(X_1X_3;Y|S_2V_2X_2.)
\end{align*}

\paragraph*{\bf Case 2, $\mathbf{\tilde{s}}_1 = \mathbf{s}_1,  \mathbf{\tilde{s}}_2 \neq  \mathbf{s}_2$}
A similar argument as in the first case gives $H(S_2|S_1) \leq I(X_2X_3;Y|S_1V_1X_1)$.

\paragraph*{\bf Case 3, $\mathbf{\tilde{s}}_1 \neq \mathbf{s}_1,  \mathbf{\tilde{s}}_2 \neq  \mathbf{s}_2, \mathbf{\tilde{s}}_1 \oplus_q \mathbf{\tilde{s}}_2=\mathbf{s}_1\oplus_q \mathbf{s}_2 $}

Using Lemma \ref{lem: prob of sG},
\begin{align*}
P\{\mathbf{v}_j=\Phi_j(\mathbf{s}_j), \tilde{\mathbf{v}}_j=\Phi_j(\tilde{\mathbf{s}}_j)~ j=1,2\} = q^{-3n} \mathbbm{1}\{ \mathbf{\tilde{v}}_1 \oplus_q \mathbf{\tilde{v}}_2=\mathbf{v}_1\oplus_q \mathbf{v}_2 \}
\end{align*}
Therefore, the above probability is nonzero only when $\mathbf{\tilde{v}}_3=\mathbf{v}_3$. Hence, as $\mathbf{s}_3=\mathbf{\tilde{s}}_3$, we get $X_3(\tilde{\mathbf{s}}_3, \tilde{\mathbf{v}}_3)=X_3(\mathbf{s}_3, \mathbf{v}_3)$. This implies that,
\begin{align*}
P\{\mathbf{x}_l=\mathbf{X}_l(\mathbf{s}_l,& \mathbf{v}_l), \tilde{\mathbf{x}}_l=\mathbf{X}_l(\tilde{\mathbf{s}}_l, \tilde{\mathbf{v}}_l) ~  l=1,2,3\}\\&=2^{-n[2H(X_1|S_1V_1)+2H(X_2|S_2V_2)+H(X_3|S_3V_3)]} \mathbbm{1}\{\mathbf{\tilde{x}}_3=\mathbf{x}_3\}.
\end{align*}

As a result,  (\ref{eq: Pe}), in this case, is simplified to :
\begin{align*}
p_{e_3}(\underline{\mathbf{s}}) \approx 2^{nH(S_1,V_1,X_1, S_2, V_2, X_2| Y S_3 V_3 X_3)} q^{-n} 2^{-n[H(X_1|S_1V_1)+H(X_2|S_2V_2)]}.
\end{align*} 

Therefore, $p_{e3}\rightarrow 0$, if $$H(S_1,V_1,X_1, S_2, V_2, X_2| Y S_3 V_3 X_3)\leq  H(X_1,X_2,V_1,V_2|S_1S_2S_3V_3X_3).$$ Using a similar argument as in the first case, this inequality is equivalent to $ H(S_1S_2|S_3) \leq I(X_1, X_2; Y| S_3V_3X_3)$.

\paragraph*{\bf Case 4, $\mathbf{\tilde{s}}_i \neq \mathbf{s}_i,  i=1,2,3 $}
Observe that,
\begin{align*}
P\{\mathbf{v}_j=\Phi_j(\mathbf{s}_j), \tilde{\mathbf{v}}_j=\Phi_j(\tilde{\mathbf{s}}_j)~ j=1,2\} &= q^{-4n}\\
P\{\mathbf{x}_l=\mathbf{X}_l(\mathbf{s}_l, \mathbf{v}_l), \tilde{\mathbf{x}}_l=\mathbf{X}_l(\tilde{\mathbf{s}}_l, \tilde{\mathbf{v}}_l) ~  l=1,2,3\}&=2^{-2n\sum_{l=1}^3 H(X_l|S_lV_l)}.
\end{align*}
Therefore,  (\ref{eq: Pe}), in this case, is simplified to $p_{e_4}(\underline{\mathbf{s}}) \approx q^{-2n}  2^{nH(  \underline{S}, \underline{V}, \underline{X}| Y)}  2^{-n\sum_{l=1}^3 H(X_l|S_lV_l)}$. As a result, one can show that $P_{e4}\rightarrow 0$, if $H(S_1S_2S_3) \leq I(X_1X_2X_3; Y)$.

Finally, note that $P_e(\underline{\mathbf{s}}) \leq \sum_{i=1}^4 P_{ei}(\underline{\mathbf{s}}).$ Moreover, $P_{ei}(\underline{\mathbf{s}})$ depends on $\underline{\mathbf{s}}$ only through its PMF. Therefore, for any typical $\underline{\mathbf{s}}$,  $P_e$ approaches zero as $n\rightarrow \infty$, if the following bounds are satisfied:
\begin{align*}
H(S_1|S_2) &\leq I(X_1 X_3;Y| S_2 V_2 X_2)\\
H(S_2|S_1) &\leq I(X_2 X_3;Y| S_1 V_1 X_1)\\
H(S_1S_2| S_1 \oplus_q S_2) & \leq I(X_1 X_2;Y| S_1 \oplus_q S_2,  V_3 X_3)\\
H(S_1,S_2) &\leq I(X_1 X_2 X_3;Y).
\end{align*}

\end{proof}

\section{Proof of Lemma \ref{lem: neigh of gamma is achievable}}\label{sec: proof_ neigh is achievable}
\begin{proof}
 For the setup in Example \ref{ex: CES is suboptimal}, the bounds given in Theorem \ref{them: achievable-rate-for -proposed scheme} are simplified to 
\begin{align}\label{eq: transmittable sources bound 1}
h(\gamma) &\leq I(X_2 X_3;Y| X_1 S_1V_1)\\\label{eq: transmittable sources bound 2}
h(\sigma) &\leq I(X_1 X_2; Y|X_3 S_3 V_3)\\\label{eq: transmittable sources bound 3}
h(\gamma)+h(\sigma)-h(\sigma * \gamma)&\leq I(X_1 X_3;Y| X_2 S_2 V_2)\\\label{eq: transmittable sources bound 4}
h(\gamma)+h(\sigma)&\leq I(X_1 X_2 X_3;Y).
\end{align}

Set $X_i=V_i, i=1,2,3$, where the distribution of these random variables are given in Theorem \ref{them: achievable-rate-for -proposed scheme}. One can verify that the source corresponding to $\sigma=0$ and $\gamma=\gamma^*$ satisfies the above inequalities and therefore can be transmitted. 

No that all the terms in (\ref{eq: transmittable sources bound 1})-(\ref{eq: transmittable sources bound 4}) are entropy functions and mutual information. Therefore, they are continuous with respect to conditional density $p(\underline{x}|\underline{s},\underline{v})$. Hence, one can show that $\forall \epsilon_0>0$, there exist a conditional density $p(\underline{x}|\underline{s},\underline{v})$  such that 
\begin{align*}
I(X_2 X_3;Y| X_1 S_1V_1)& \geq 2-H(N)-\eta(\epsilon_0)\\
I(X_1 X_2; Y|X_3 S_3 V_3)&\geq \epsilon_0\\
I(X_1 X_3;Y| X_2 S_2 V_2)&\geq 2-H(N)-\eta(\epsilon_0)\\
I(X_1 X_2 X_3;Y) &\geq 2-H(N)-\eta(\epsilon_0),
\end{align*}
where $\eta()$ is function of $\epsilon$ such that $\eta(\epsilon)\rightarrow 0$ as $\epsilon \rightarrow 0$.

Note also that the left-hand sides in (\ref{eq: transmittable sources bound 1})-(\ref{eq: transmittable sources bound 4}) are continuous in $\sigma$ and $\gamma$. Hence $\exists \epsilon'>0$ such that when $\sigma\leq \epsilon', |\gamma-\gamma^*| \leq \epsilon'$, we have 
\begin{align*}
h(\gamma)&\leq 2-H(N)-\eta(\epsilon_0)\\
h(\sigma) &\leq \epsilon_0\\
h(\gamma)+h(\sigma)-h(\sigma * \gamma)&\leq 2-H(N)-\eta(\epsilon_0)\\
h(\gamma)+h(\sigma) &\leq 2-H(N)-\eta(\epsilon_0)
\end{align*}

This implies that the source corresponding to $\sigma\leq \epsilon', \gamma\leq \gamma^*-\epsilon'$ can be transmitted reliably and the proof is complete.
\end{proof}
